# Supplementary material for: Value Functions for Depth-Limited Solving in Zero-Sum Imperfect-Information Games
Source: arXiv:1906.06412 source file (2022-03-24)
Supplement: Supplementary file 1 [file appendix_lossexpl.tex]

\subsection{Loss vs. Exploitability}\label{sec:app:lossexpl}

% \vknote{This subsection is missing an introduction.}
This subsection presents the results of the loss vs exploitability experiment described in Section \ref{sec:experiments} for all domains, each time showing two separate neural network training cycles.

The x-axis denotes the network error, while the y-axis denotes the normalized exploitability after 1000 iterations of \DLCFR using
the network with that corresponding error.

\begin{figure}[H]
\centering
\includegraphics[width=\linewidth]{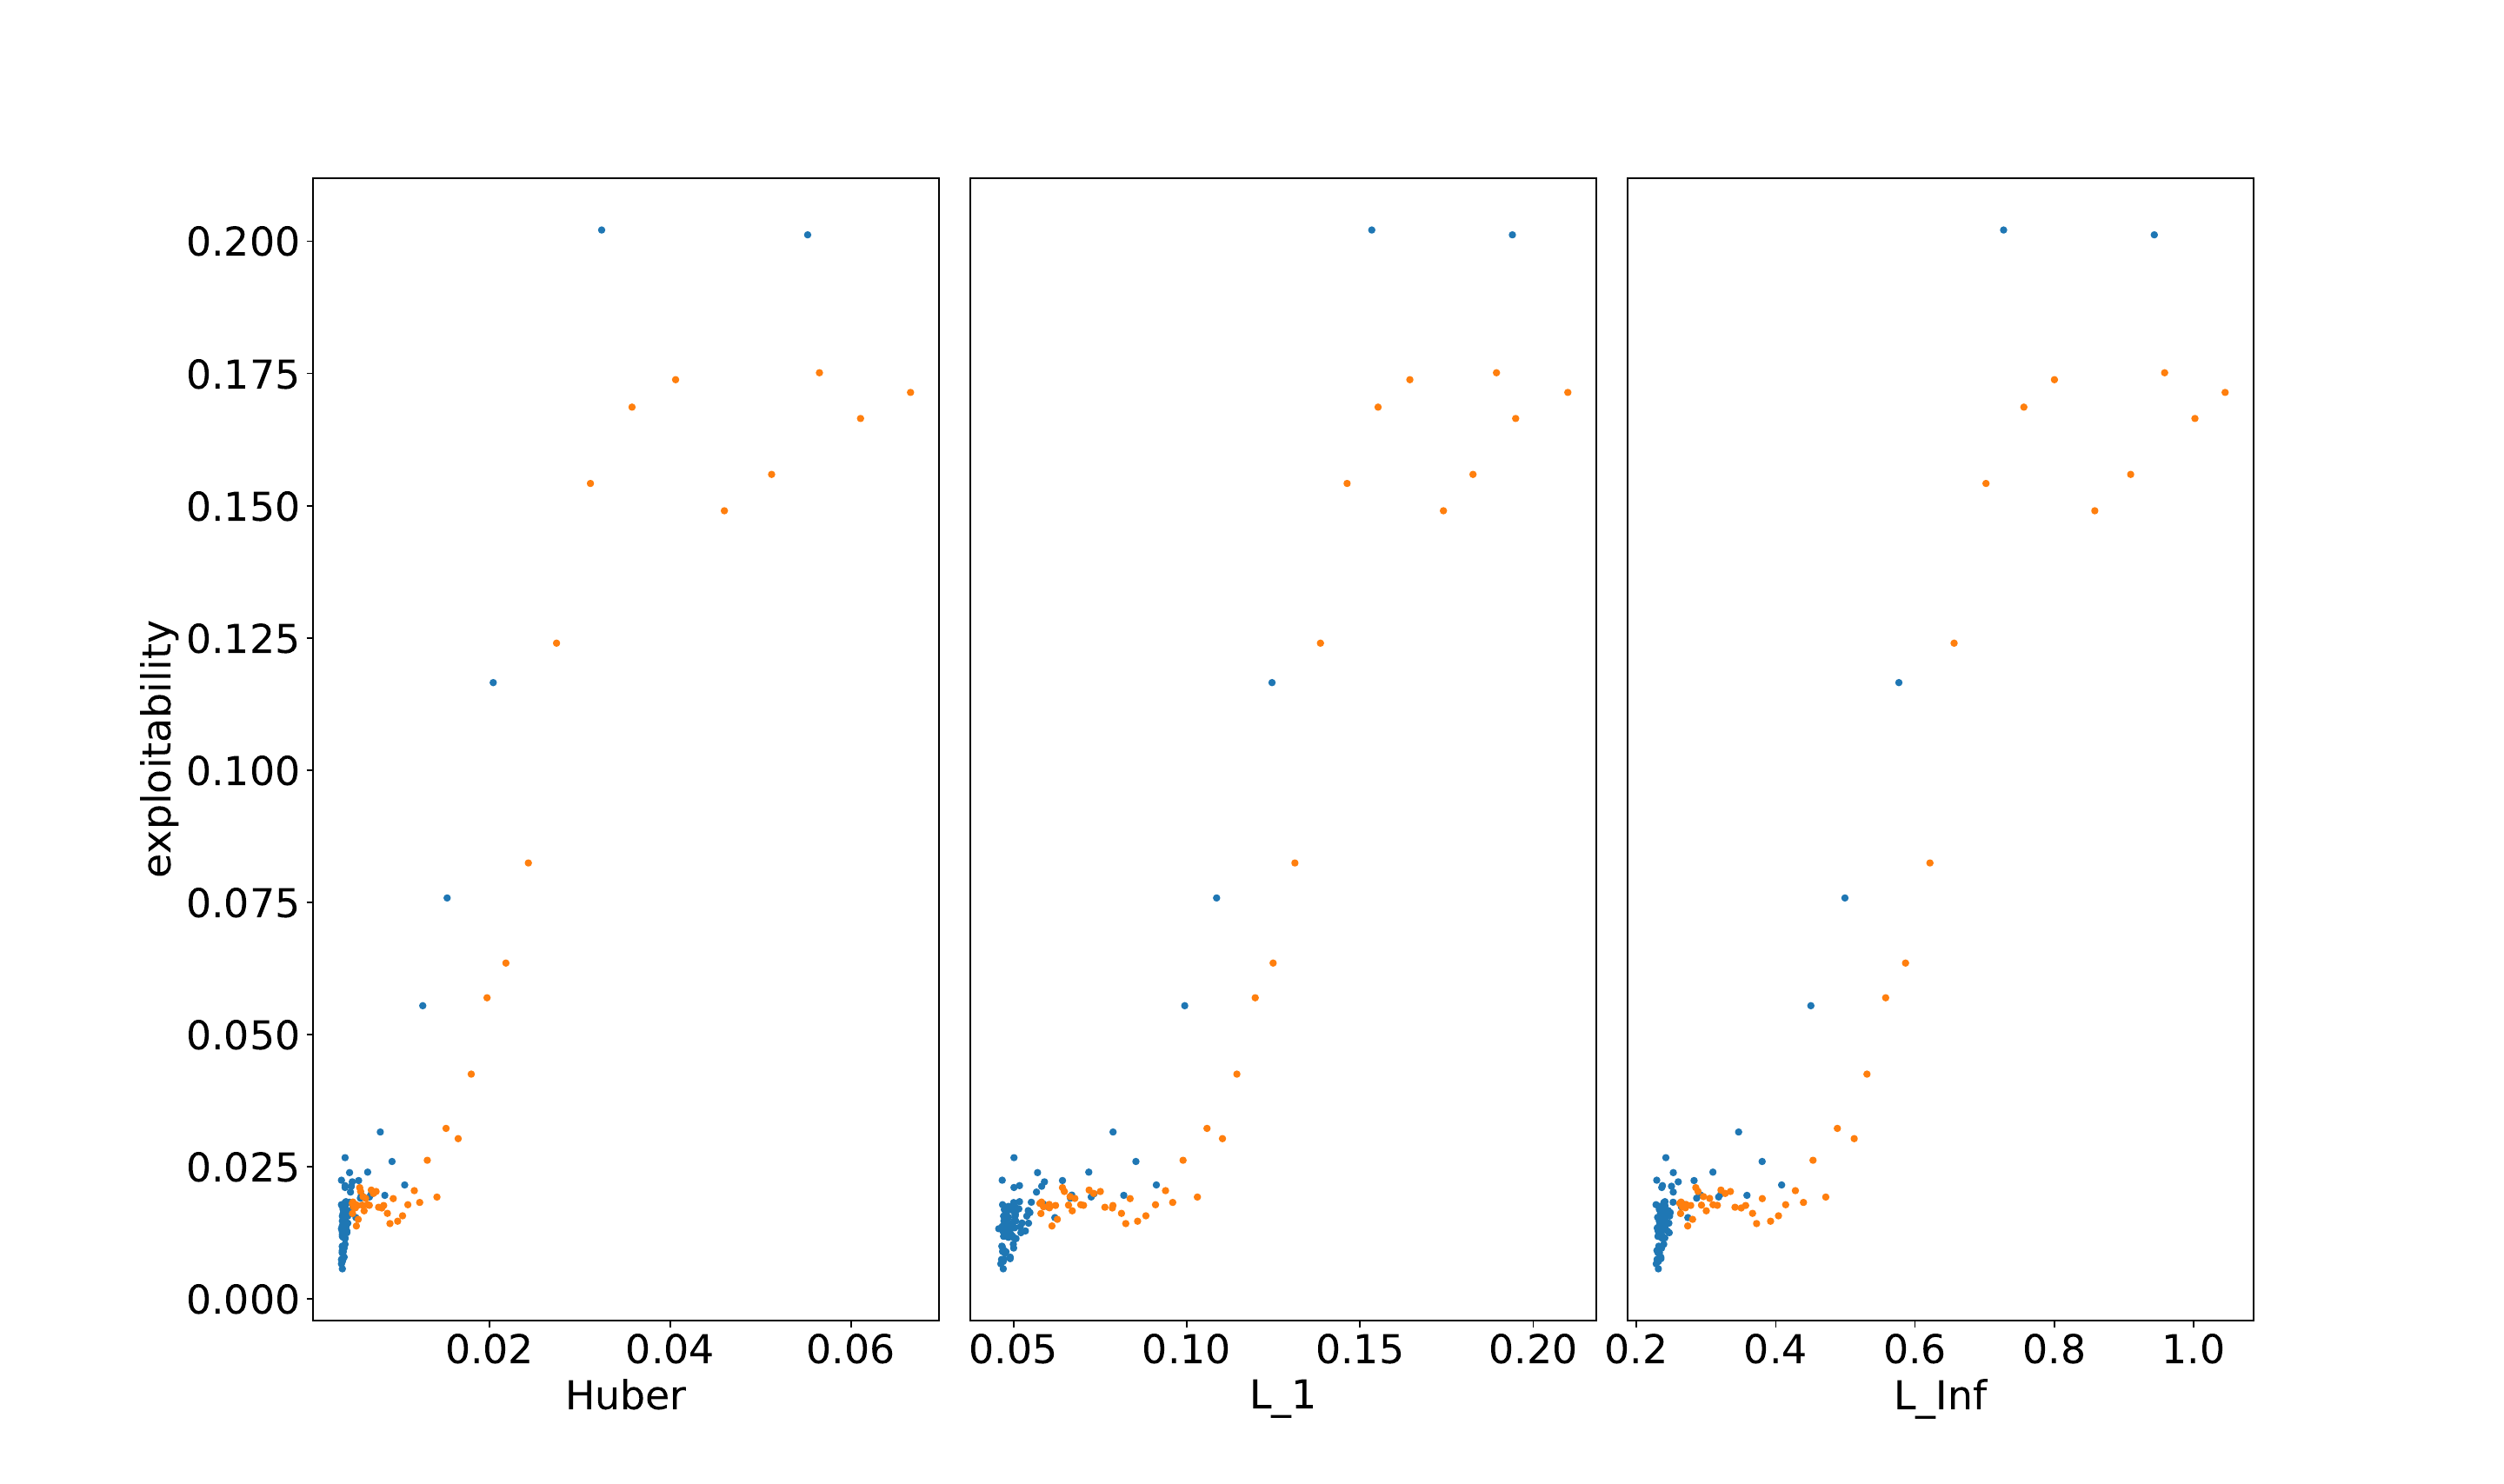}\hfill
\caption{Exploitability vs validation error in Goofspiel. The blue and orange lines correspond to two different neural network training cycles with
different parameter settings.}
\end{figure}

\begin{figure}[H]
\centering
\includegraphics[width=\linewidth]{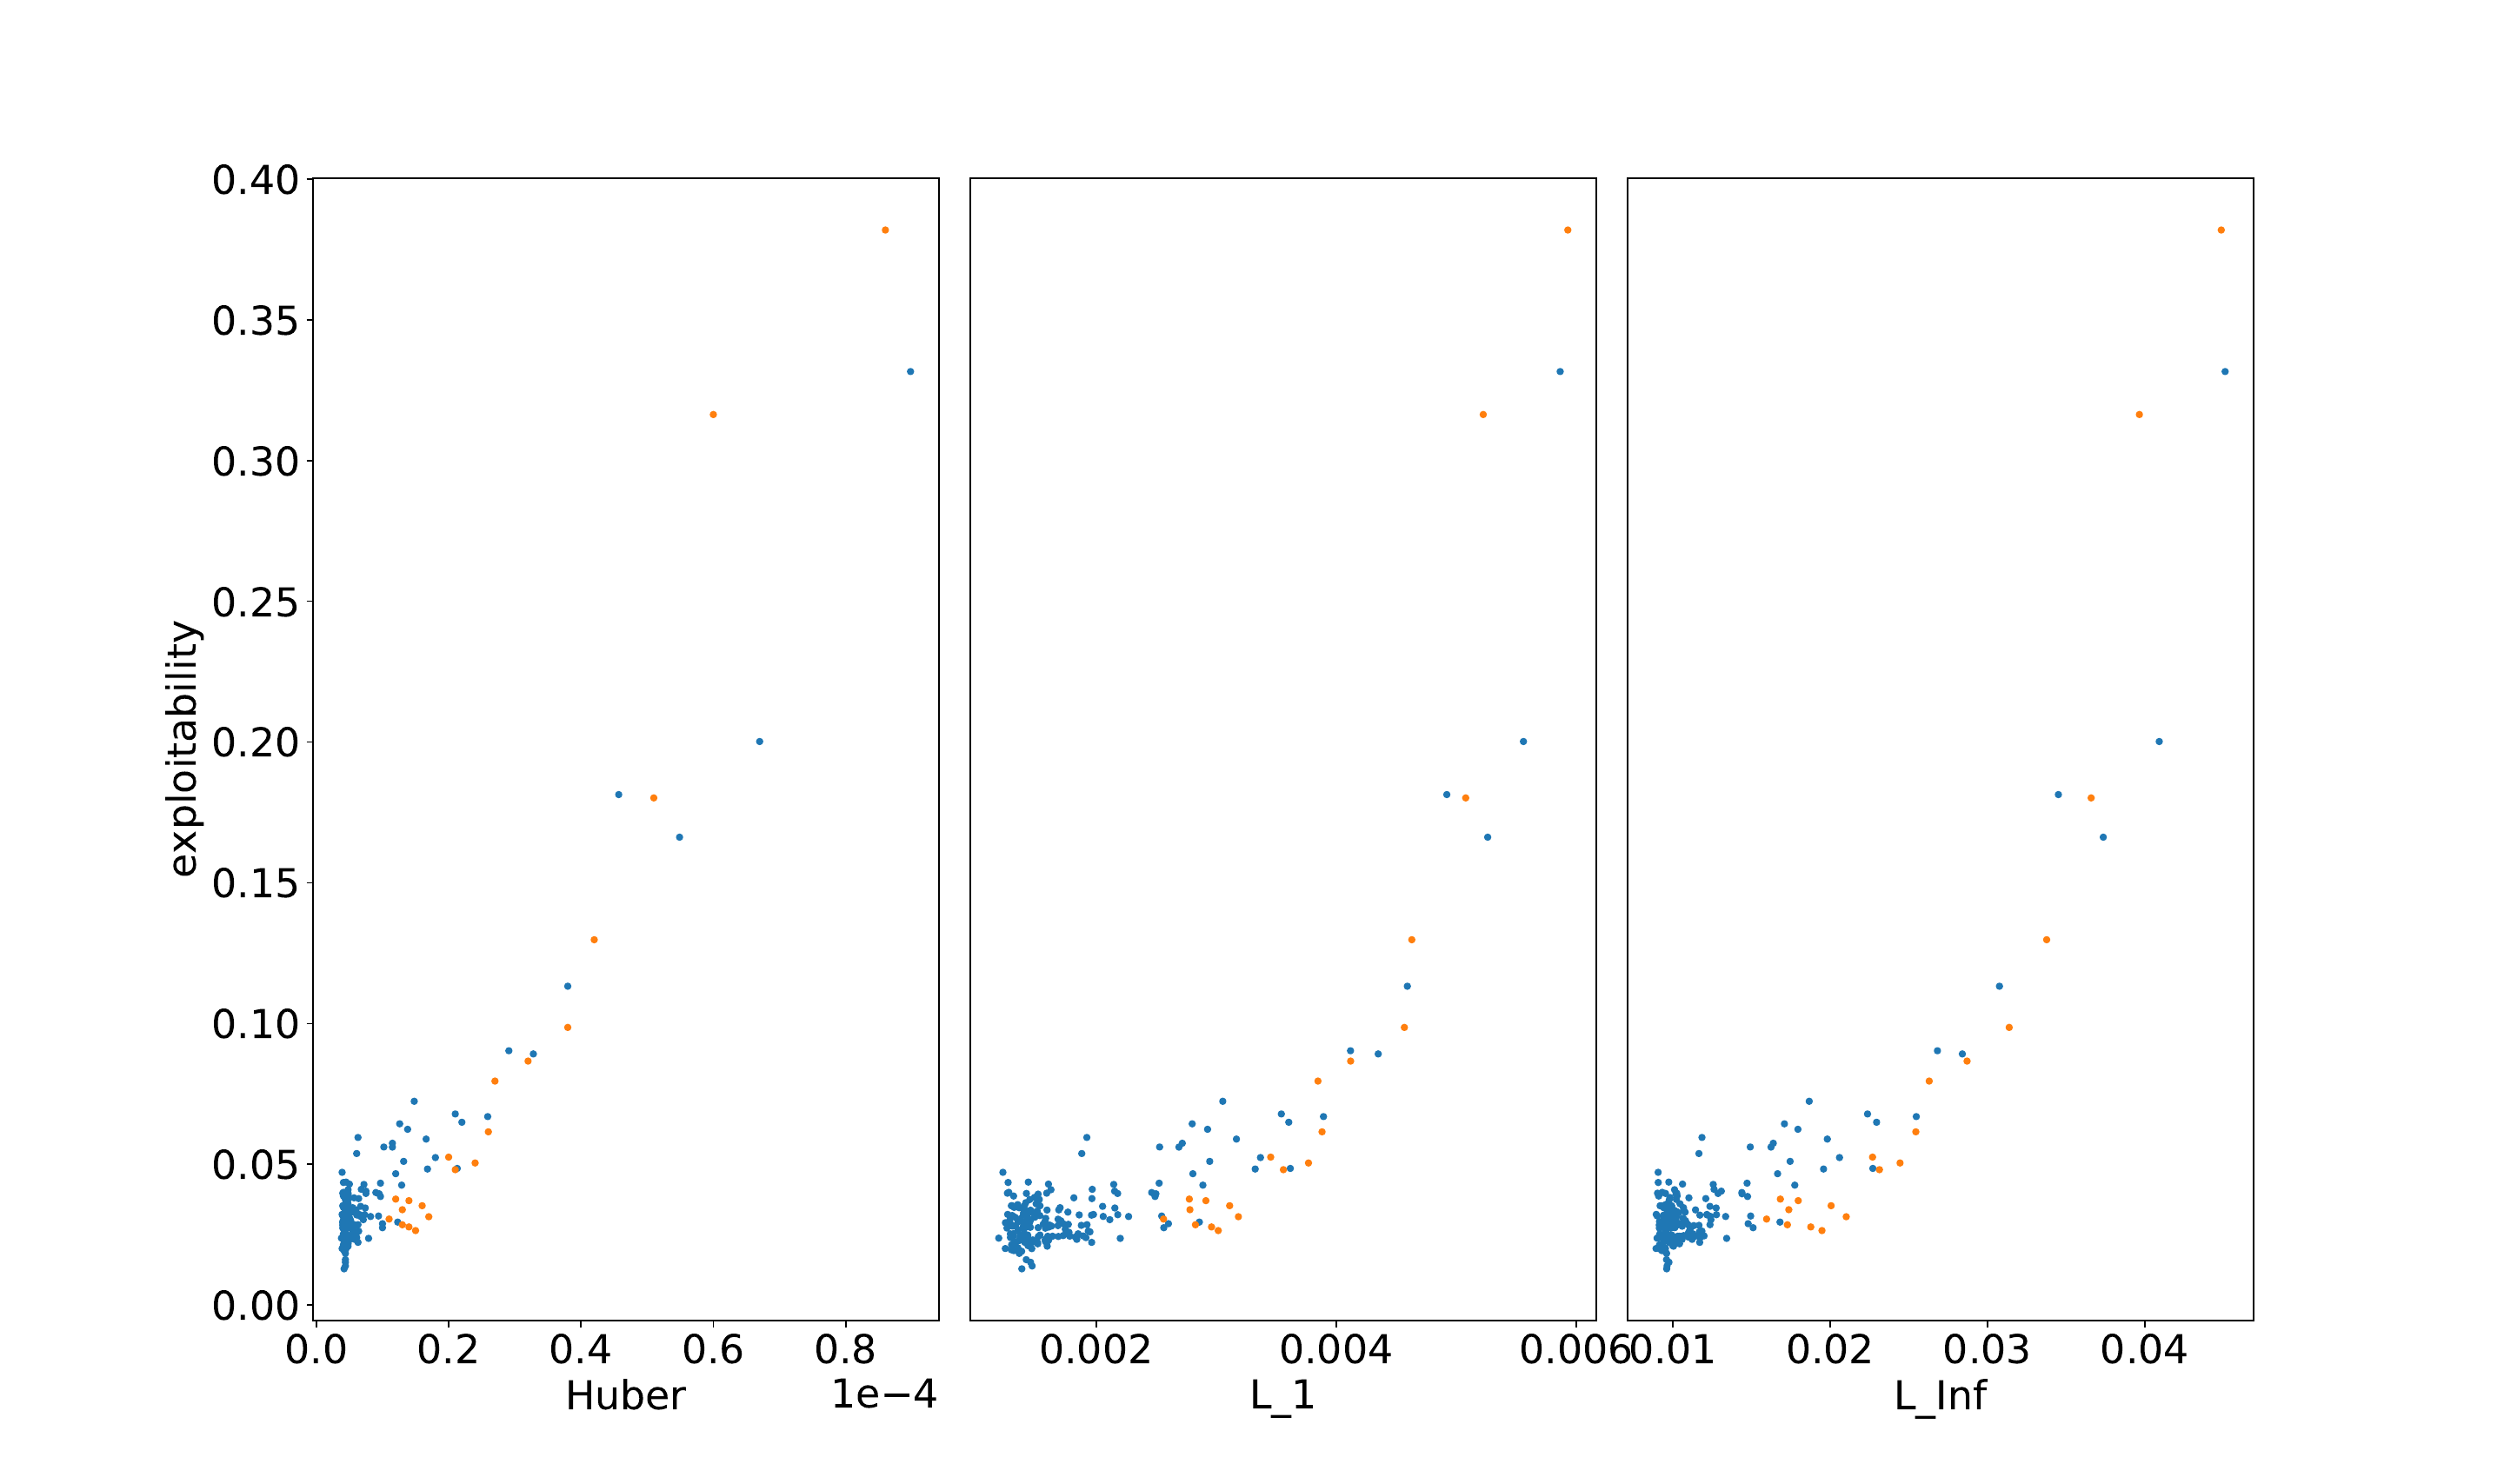}\hfill
\caption{Exploitability vs validation error in OZ. The blue and orange lines correspond to two different neural network training cycles with
different parameter settings.}
\end{figure}

\begin{figure}[H]
\centering
\includegraphics[width=\linewidth]{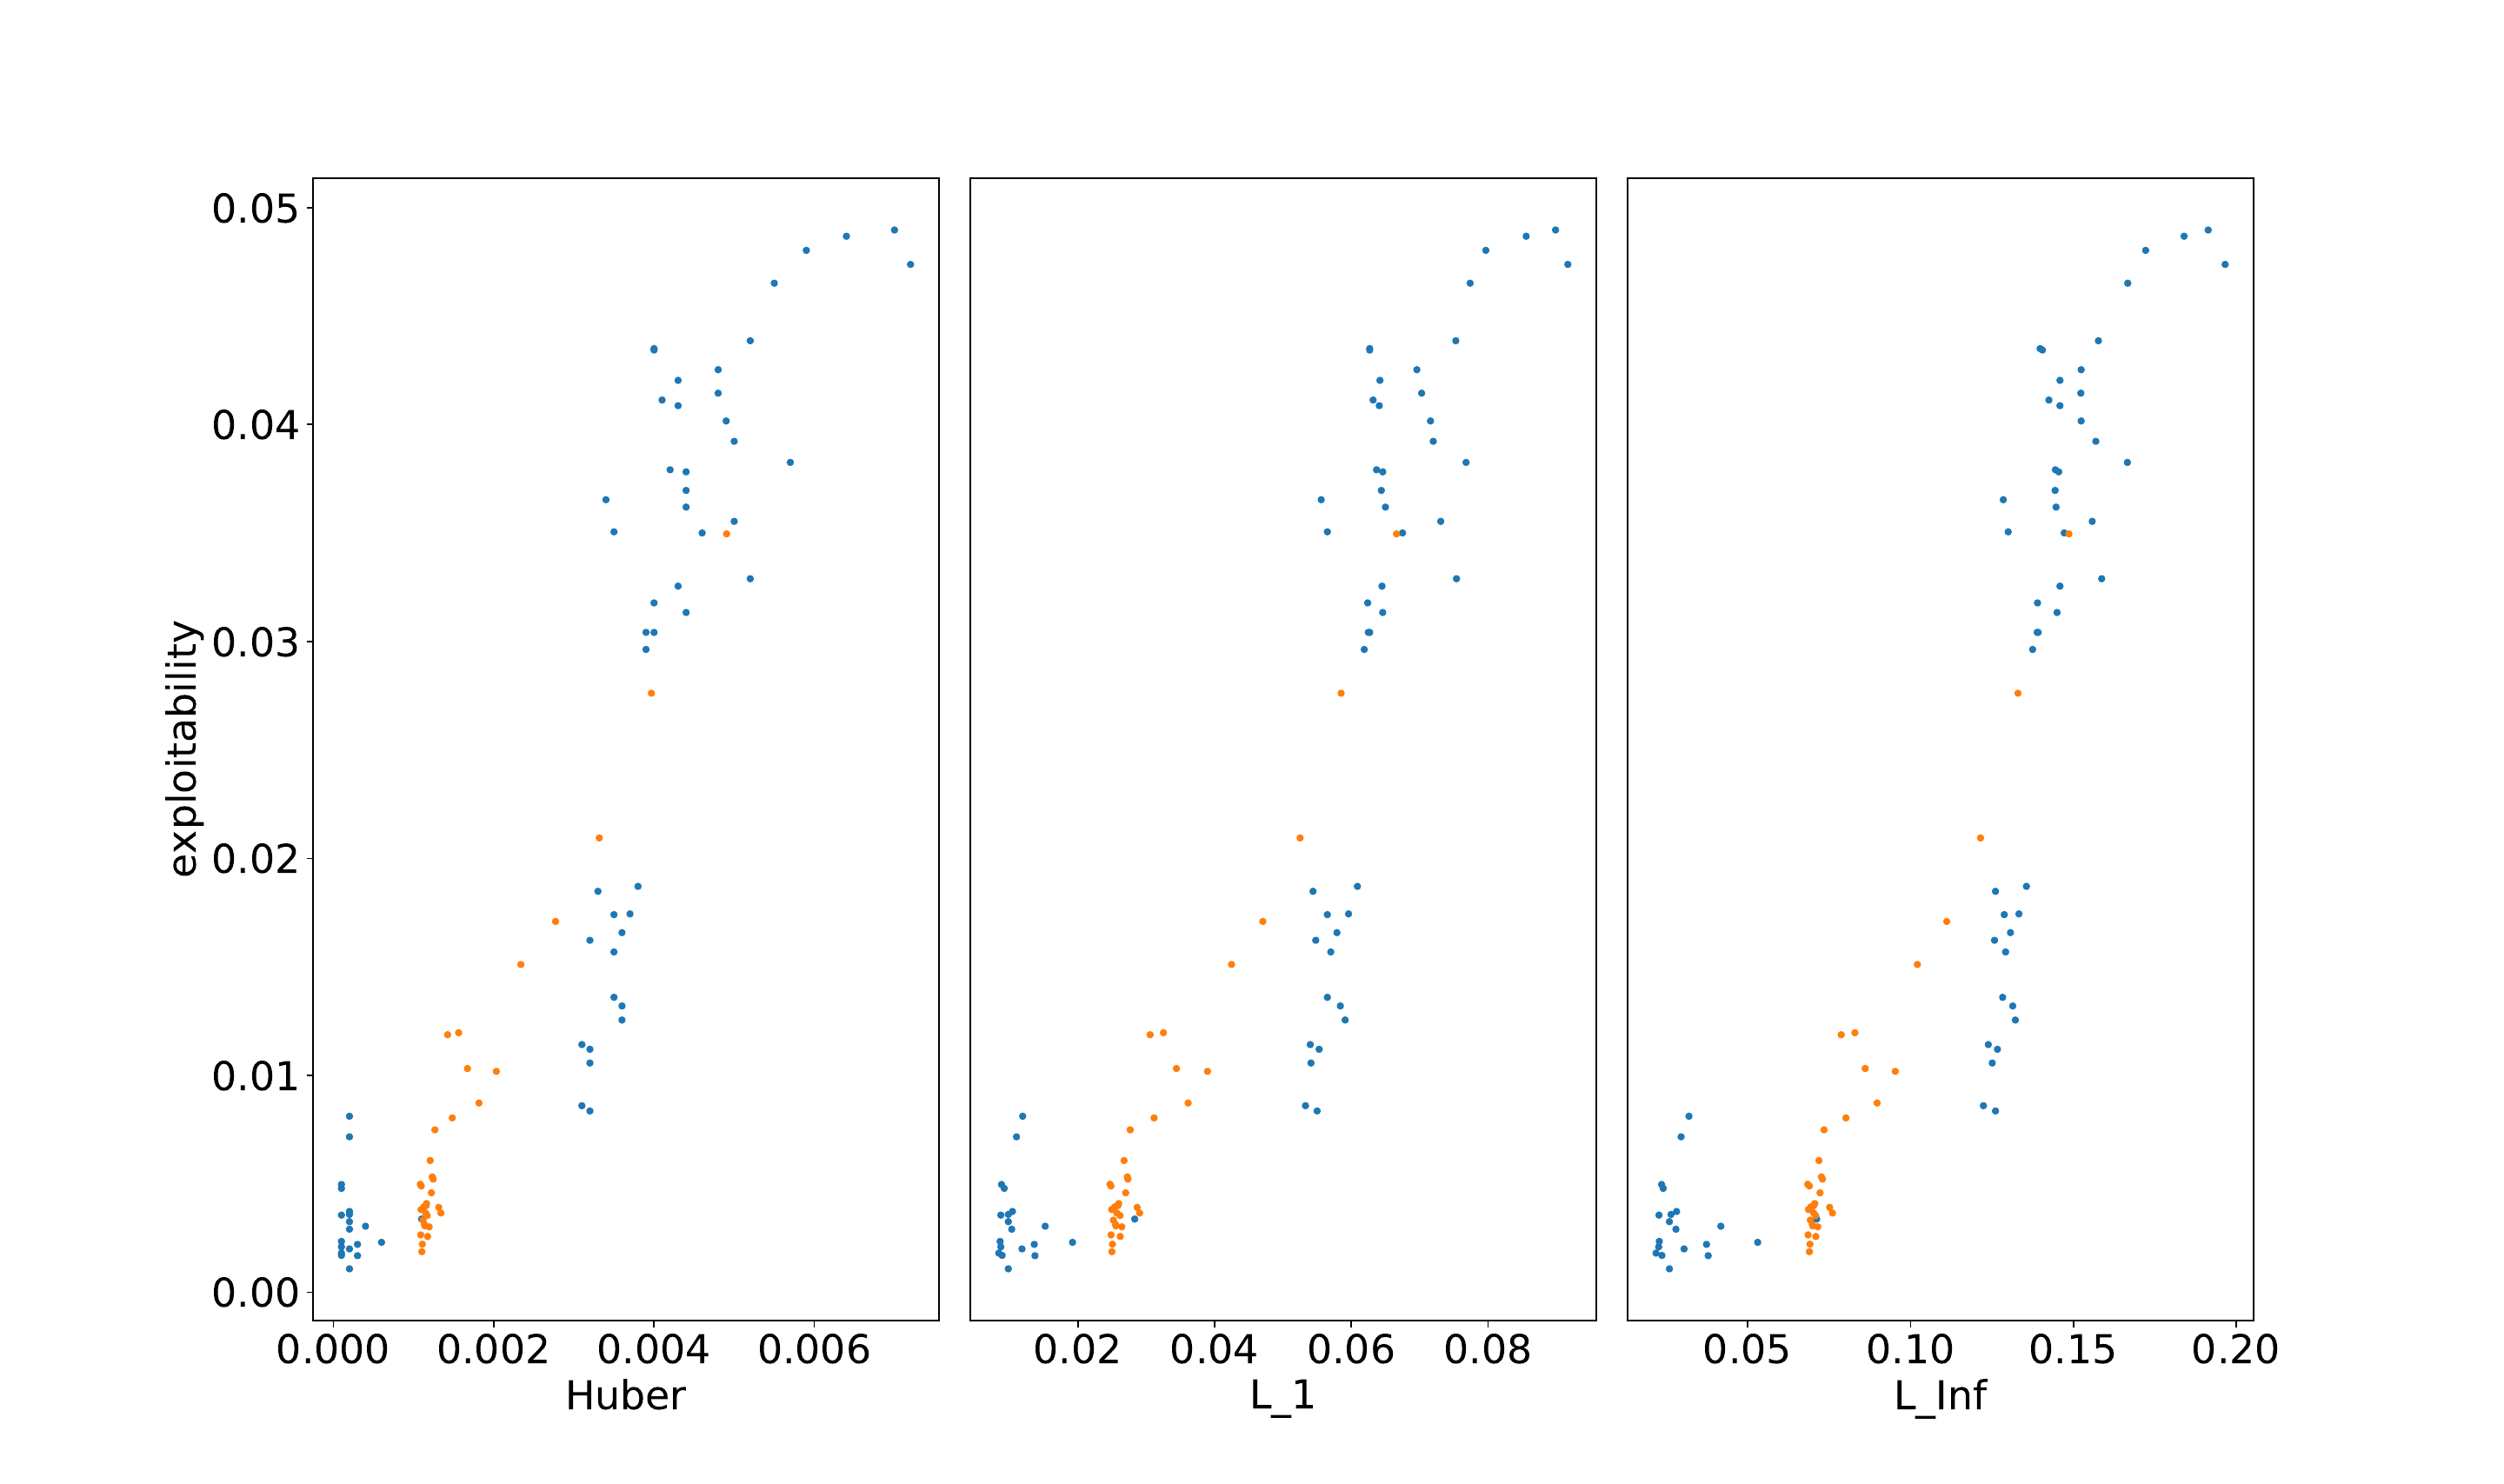}\hfill
\caption{Exploitability vs validation error in GP. Blue denotes a neural network training cycle where validation loss has been measured after each batch to get more insight about the relationship in high error regions.
Orange denotes errors after each epoch. Both networks use a different seed for initial parameter initializations.}
\end{figure}

We are able to achieve exploitability below 0.01 in all three domains.
In case of GP we initially observed very fast convergence due to smaller input size compared to OZ and II-GS.
We therefore opted to investigate how the relationship between error and exploitability behaves in very early stages of training by
calculating the validation error after each batch update. Convergence with batches shows to be noisier as in epochs but eventually
reaches the same performance.
